# Supplementary material for: Deep Keypoint-Based Camera Pose Estimation with Geometric Constraints
Source: arXiv:2007.15122 source file (2020-07-29)
Supplement: Supplementary file 1 [file supp_ablation_apolloModels.tex]

%%%%% apollo model on apollo
\begin{table*}[h]
    \scriptsize
    \centering
    \begin{tabular}{lllllllllllllll}
        \toprule
        \multirow{2}{*} {Apollo dataset} & \multicolumn{7}{c}{Rotation (inlier ratio, error median)} & \multicolumn{7}{c}{Translation (inlier ratio, error median)} \\
        \cmidrule(r){2-8} \cmidrule(r){9-15} \\
         Apollo Models & 0.01 & 0.02 & 0.05 & 0.1 & 0.5 & Mean & Med. & 0.1 & 0.2 & 0.5 & 1.0 & 2.0 & Mean & Med. \\
        \midrule
  
Base(Si-Ran) & 0.058 & 0.227 & 0.662 & 0.922 & 0.997 & 0.157 & 0.037 & 0.065 & 0.214 & 0.623 & 0.890 & 0.979 & 0.788 & 0.388
\\ \hline
Base(Sp-Ran) & 0.000 & 0.007 & 0.090 & 0.355 & 0.952 & 0.202 & 0.128 & 0.003 & 0.011 & 0.061 & 0.213 & 0.524 & 4.816 & 1.899
\\ \hline
Si-Df-f & 0.069 & 0.239 & 0.670 & 0.912 & 0.997 & 0.079 & 0.036 & 0.126 & 0.338 & 0.719 & 0.884 & 0.954 & 0.745 & 0.293
\\ \hline
Si-Df-p & 0.110 & 0.308 & 0.729 & 0.942 & 0.997 & 0.097 & 0.031 & 0.216 & 0.506 & 0.850 & 0.953 & 0.987 & 0.455 & 0.197
\\ \hline
Sp-Df-f & 0.013 & 0.078 & 0.483 & 0.860 & 0.996 & 0.096 & 0.051 & 0.027 & 0.099 & 0.428 & 0.784 & 0.944 & 0.972 & 0.573
\\ \hline
Sp-Df-p & 0.014 & 0.088 & 0.499 & 0.865 & 0.997 & 0.094 & 0.050 & 0.041 & 0.139 & 0.520 & 0.836 & 0.961 & 0.855 & 0.483
\\ \hline
Ours(Sp-Df-f-end) & 0.012 & 0.098 & 0.553 & 0.900 & 0.999 & 0.086 & 0.046 & 0.044 & 0.144 & 0.560 & 0.876 & 0.970 & 0.769 & 0.451
\\ \hline
Ours(Sp-Df-p-end) & 0.018 & 0.107 & 0.580 & 0.905 & 0.998 & 0.085 & 0.044 & 0.047 & 0.178 & 0.637 & 0.903 & 0.975 & 0.708 & 0.398
\\ \hline
Ours(Sp-Df-fp-end) & 0.020 & 0.117 & 0.593 & 0.910 & 0.999 & 0.084 & 0.043 & 0.042 & 0.149 & 0.555 & 0.881 & 0.977 & 0.714 & 0.454
\\ \hline

Sp-D-a-p-b16 & 0.012 & 0.077 & 0.496 & 0.865 & 0.998 & 0.091 & 0.050 & 0.034 & 0.124 & 0.502 & 0.850 & 0.964 & 1.052 & 0.497
\\ \hline

Si-D-a-p-b4 & 0.061 & 0.215 & 0.623 & 0.888 & 0.995 & 0.122 & 0.039 & 0.093 & 0.283 & 0.634 & 0.831 & 0.931 & 0.936 & 0.353
\\ \hline
Sp-D-end-a-p-b12 & 0.020 & 0.111 & 0.565 & 0.900 & 0.999 & 0.086 & 0.046 & 0.049 & 0.172 & 0.599 & 0.896 & 0.977 & 0.805 & 0.421
\\ \hline

Sp-D-f-b12 & 0.012 & 0.088 & 0.508 & 0.876 & 0.999 & 0.089 & 0.049 & 0.037 & 0.130 & 0.489 & 0.828 & 0.962 & 1.050 & 0.509
\\ \hline
Sp-D-f-end-b8 & 0.021 & 0.124 & 0.592 & 0.914 & 0.999 & 0.084 & 0.044 & 0.044 & 0.154 & 0.576 & 0.884 & 0.976 & 0.774 & 0.443
\\ \hline

% Si-Ran & 0.054 & 0.226 & 0.662 & 0.922 & 0.996 & 0.151 & 0.036 & 0.066 & 0.220 & 0.629 & 0.895 & 0.978 & 0.878 & 0.385
% \\ \hline
% Sp-Ran & 0.001 & 0.007 & 0.074 & 0.337 & 0.951 & 0.225 & 0.133 & 0.003 & 0.010 & 0.061 & 0.201 & 0.491 & 5.249 & 2.041
% \\ \hline
% Si-Df-f & 0.108 & 0.323 & 0.751 & 0.952 & 0.997 & 0.076 & 0.029 & 0.217 & 0.526 & 0.889 & 0.974 & 0.991 & 0.452 & 0.190
% \\ \hline
% Si-Df-p & 0.085 & 0.274 & 0.707 & 0.932 & 0.994 & 0.092 & 0.033 & 0.171 & 0.441 & 0.810 & 0.940 & 0.980 & 0.664 & 0.226
% \\ \hline
% Si-Df-fp & 0.133 & 0.350 & 0.765 & 0.952 & 0.998 & 0.062 & 0.028 & 0.324 & 0.672 & 0.946 & 0.985 & 0.993 & 0.343 & 0.144
% \\ \hline
% Sp-Df-f & 0.013 & 0.091 & 0.509 & 0.877 & 0.997 & 0.087 & 0.049 & 0.027 & 0.106 & 0.462 & 0.803 & 0.951 & 0.922 & 0.535
% \\ \hline
% Sp-Df-p & 0.013 & 0.105 & 0.554 & 0.893 & 0.997 & 0.088 & 0.046 & 0.042 & 0.155 & 0.587 & 0.888 & 0.973 & 0.763 & 0.434
% \\ \hline
% Sp-Df-f-end & 0.014 & 0.100 & 0.553 & 0.889 & 0.998 & 0.089 & 0.046 & 0.038 & 0.135 & 0.550 & 0.866 & 0.964 & 0.752 & 0.457
% \\ \hline
% % Sp-Df-p-end & 0.001 & 0.006 & 0.051 & 0.226 & 0.888 & 0.273 & 0.187 & 0.004 & 0.018 & 0.087 & 0.276 & 0.551 & 3.457 & 1.756
% % \\ \hline
% Sp-Df-p-end & 0.018 & 0.109 & 0.575 & 0.902 & 0.998 & 0.088 & 0.044 & 0.053 & 0.190 & 0.651 & 0.917 & 0.980 & 0.761 & 0.385
% \\ \hline
% Sp-Df-fp-end & 0.017 & 0.125 & 0.592 & 0.915 & 0.999 & 0.067 & 0.043 & 0.058 & 0.206 & 0.676 & 0.931 & 0.983 & 0.669 & 0.367
% \\ \hline

\bottomrule
    \end{tabular}
\caption{\label{tab:exp_ablation_ref_table} \textbf{Apollo model on Apollo dataset. The full table for rotation and translation error.} The set of models are trained in solely in KITTI dataset or ApolloScape dataset. }
\end{table*}

%%%% apollo models on kitti
\begin{table*}[h]
    \scriptsize
    \centering
    \begin{tabular}{lllllllllllllll}
        \toprule
        \multirow{2}{*} {Apollo dataset} & \multicolumn{7}{c}{Rotation (inlier ratio, error median)} & \multicolumn{7}{c}{Translation (inlier ratio, error median)} \\
        \cmidrule(r){2-8} \cmidrule(r){9-15} \\
         Apollo Models & 0.01 & 0.02 & 0.05 & 0.1 & 0.5 & Mean & Med. & 0.1 & 0.2 & 0.5 & 1.0 & 2.0 & Mean & Med. \\
        \midrule
Base(Si-Ran) & 0.011 & 0.068 & 0.427 & 0.816 & 0.997 & 0.456 & 0.057 & 0.024 & 0.084 & 0.390 & 0.735 & 0.900 & 1.980 & 0.613
\\ \hline
Base(Sp-Ran) & 0.000 & 0.006 & 0.031 & 0.102 & 0.627 & 1.178 & 0.367 & 0.001 & 0.005 & 0.033 & 0.114 & 0.304 & 11.085 & 3.330
\\ \hline
Si-Df-f & 0.010 & 0.056 & 0.365 & 0.706 & 0.964 & 0.130 & 0.066 & 0.022 & 0.074 & 0.362 & 0.663 & 0.824 & 3.133 & 0.686
\\ \hline
Si-Df-p & 0.015 & 0.091 & 0.449 & 0.786 & 0.980 & 0.096 & 0.054 & 0.018 & 0.075 & 0.392 & 0.725 & 0.860 & 1.932 & 0.606
\\ \hline
Sp-Df-f & 0.000 & 0.003 & 0.029 & 0.124 & 0.693 & 0.426 & 0.313 & 0.001 & 0.006 & 0.033 & 0.122 & 0.308 & 4.695 & 3.365
\\ \hline
Sp-Df-p & 0.000 & 0.003 & 0.028 & 0.113 & 0.718 & 0.413 & 0.311 & 0.001 & 0.005 & 0.032 & 0.116 & 0.303 & 5.227 & 3.509
\\ \hline
Ours(Sp-Df-f-end) & 0.001 & 0.008 & 0.059 & 0.217 & 0.904 & 0.248 & 0.194 & 0.000 & 0.006 & 0.057 & 0.231 & 0.510 & 3.070 & 1.954
\\ \hline
Ours(Sp-Df-p-end) & 0.001 & 0.008 & 0.064 & 0.279 & 0.960 & 0.198 & 0.161 & 0.005 & 0.013 & 0.089 & 0.309 & 0.617 & 2.614 & 1.554
\\ \hline
Ours(Sp-Df-fp-end) & 0.003 & 0.012 & 0.110 & 0.353 & 0.962 & 0.177 & 0.132 & 0.004 & 0.013 & 0.086 & 0.328 & 0.649 & 2.352 & 1.435
\\ \hline

Sp-D-a-p-b16 & 0.002 & 0.013 & 0.138 & 0.424 & 0.956 & 0.170 & 0.118 & 0.007 & 0.028 & 0.149 & 0.422 & 0.699 & 2.442 & 1.190
\\ \hline

Si-D-a-p-b4 & 0.012 & 0.067 & 0.347 & 0.667 & 0.946 & 0.154 & 0.069 & 0.017 & 0.071 & 0.303 & 0.597 & 0.773 & 2.795 & 0.779
\\ \hline
Sp-D-end-a-p-b12 & 0.004 & 0.019 & 0.169 & 0.467 & 0.973 & 0.159 & 0.106 & 0.006 & 0.025 & 0.152 & 0.443 & 0.750 & 2.466 & 1.112
\\ \hline
Sp-D-f-b12 & 0.001 & 0.017 & 0.151 & 0.454 & 0.957 & 0.173 & 0.110 & 0.008 & 0.028 & 0.147 & 0.406 & 0.684 & 3.068 & 1.239
\\ \hline
Sp-D-f-end-b8 & 0.004 & 0.021 & 0.185 & 0.529 & 0.978 & 0.135 & 0.094 & 0.006 & 0.029 & 0.182 & 0.485 & 0.767 & 2.454 & 1.032
\\ \hline
        
% Si-Ran & 0.011 & 0.068 & 0.427 & 0.816 & 0.997 & 0.456 & 0.057 & 0.024 & 0.083 & 0.390 & 0.735 & 0.900 & 2.061 & 0.613
% \\ \hline
% Sp-Ran & 0.000 & 0.003 & 0.027 & 0.121 & 0.719 & 0.935 & 0.291 & 0.001 & 0.007 & 0.046 & 0.152 & 0.378 & 7.607 & 2.736
% \\ \hline
% Si-Df-f & 0.011 & 0.078 & 0.435 & 0.755 & 0.960 & 0.125 & 0.057 & 0.018 & 0.072 & 0.352 & 0.683 & 0.832 & 2.600 & 0.660
% \\ \hline
% Si-Df-p & 0.011 & 0.057 & 0.336 & 0.652 & 0.954 & 0.156 & 0.071 & 0.013 & 0.068 & 0.313 & 0.663 & 0.838 & 2.457 & 0.693
% \\ \hline
% Si-Df-fp & 0.016 & 0.085 & 0.439 & 0.747 & 0.970 & 0.112 & 0.057 & 0.019 & 0.078 & 0.339 & 0.673 & 0.824 & 2.267 & 0.692
% \\ \hline
% Sp-Df-f & 0.001 & 0.010 & 0.095 & 0.354 & 0.952 & 0.204 & 0.133 & 0.004 & 0.014 & 0.098 & 0.314 & 0.621 & 3.337 & 1.537
% \\ \hline
% Sp-Df-p & 0.000 & 0.006 & 0.062 & 0.268 & 0.925 & 0.229 & 0.161 & 0.005 & 0.015 & 0.100 & 0.296 & 0.609 & 3.749 & 1.577
% \\ \hline
(old)Sp-Df-f-end & 0.001 & 0.009 & 0.087 & 0.305 & 0.932 & 0.214 & 0.149 & 0.003 & 0.014 & 0.097 & 0.314 & 0.601 & 3.073 & 1.548
\\ \hline

% Sp-Df-p-end & 0.001 & 0.003 & 0.055 & 0.235 & 0.891 & 0.275 & 0.186 & 0.004 & 0.014 & 0.089 & 0.268 & 0.557 & 3.740 & 1.712
% \\ \hline
(old)Sp-Df-p-end & 0.000 & 0.004 & 0.030 & 0.166 & 0.833 & 0.393 & 0.229 & 0.002 & 0.007 & 0.060 & 0.207 & 0.492 & 4.181 & 2.046
\\ \hline
(old)Sp-Df-fp-end & 0.001 & 0.008 & 0.104 & 0.373 & 0.967 & 0.174 & 0.128 & 0.004 & 0.019 & 0.112 & 0.371 & 0.674 & 2.496 & 1.318
\\ \hline

\bottomrule
    \end{tabular}
\caption{\label{tab:exp_ablation_ref_table} \textbf{Apollo model on KITTI dataset. The full table for rotation and translation error.} The set of models are trained in solely in KITTI dataset or ApolloScape dataset. }
\end{table*}
