# Supplementary material for: Deep Keypoint-Based Camera Pose Estimation with Geometric Constraints
Source: arXiv:2007.15122 source file (2020-07-29)
Supplement: Supplementary file 2 [file supp_ablation_kittiModels.tex]

%%%%% kitti model on KITTI
\begin{table*}[h]
    \scriptsize
    \centering
    \begin{tabular}{llllllllllllllll}
        \toprule
        \multicolumn{2}{c}{\multirow{2}{*} {KITTI dataset}} & \multicolumn{7}{c}{Rotation (inlier ratio, error median)} & \multicolumn{7}{c}{Translation (inlier ratio, error median)} \\
        \cmidrule(r){3-9} \cmidrule(r){10-16} \\
        Catogories & KITTI Models & 0.01 & 0.02 & 0.05 & 0.1 & 0.5 & Mean & Med. & 0.1 & 0.2 & 0.5 & 1.0 & 2.0 & Mean & Med. \\
        \midrule

\textbf{Si-base} 
& Si-Ran & 0.017 & 0.078 & 0.433 & 0.818 & 0.997 & 0.391 & 0.056 & 0.020 & 0.085 & 0.372 & 0.727 & 0.899 & 1.895 & 0.639
\\ \midrule % \hline
\textbf{Sp-base} 
& Sp-Ran & 0.001 & 0.004 & 0.048 & 0.189 & 0.815 & 0.641 & 0.217 & 0.003 & 0.014 & 0.077 & 0.222 & 0.481 & 5.798 & 2.103
\\ \midrule % \hline
\textbf{Si-models} 
& Si-Df-f & 0.028 & 0.143 & 0.645 & 0.938 & 0.998 & 0.051 & 0.041 & 0.032 & 0.137 & 0.517 & 0.812 & 0.914 & 1.699 & 0.484
\\  % \hline
& Si-Df-p & 0.028 & 0.125 & 0.579 & 0.901 & 0.995 & 0.059 & 0.044 & 0.025 & 0.119 & 0.485 & 0.787 & 0.903 & 1.472 & 0.513
\\ % \hline
& Si-Df-fp & 0.028 & 0.161 & 0.680 & 0.947 & 0.998 & 0.111 & 0.038 & 0.037 & 0.135 & 0.519 & 0.816 & 0.916 & 1.741 & 0.484
\\ \midrule % \hline
\textbf{Sp-models} 
& Sp-Df-f & 0.005 & 0.034 & 0.263 & 0.633 & 0.997 & 0.100 & 0.078 & 0.009 & 0.048 & 0.258 & 0.579 & 0.830 & 1.476 & 0.846
\\ % \hline
& Sp-Df-p & 0.023 & 0.100 & 0.527 & 0.875 & 0.996 & 0.130 & 0.047 & 0.025 & 0.108 & 0.454 & 0.770 & 0.887 & 1.719 & 0.539
\\ \midrule % \hline
\texttt{DeepFEPE} 
& Sp-Df-f-end & 0.023 & 0.144 & 0.614 & 0.915 & 0.998 & 0.053 & 0.042 & 0.033 & 0.114 & 0.511 & 0.800 & 0.905 & 1.662 & 0.489
\\ 
& Sp-Df-p-end & 0.021 & 0.142 & 0.613 & 0.932 & 1.000 & 0.050 & 0.041 & 0.029 & 0.119 & 0.498 & 0.798 & 0.905 & 1.600 & 0.503
\\ 
& Sp-Df-fp-end & 0.018 & 0.103 & 0.535 & 0.910 & 1.000 & 0.054 & 0.048 & 0.037 & 0.131 & 0.498 & 0.805 & 0.917 & 1.062 & 0.504
\\ \hline

 \bottomrule % \hline
\end{tabular} 

\caption{\label{tab:exp_ablation_ref_table} \textbf{KITTI model on KITTI dataset. The full table for rotation and translation error.} The set of models are trained in solely in KITTI dataset or ApolloScape dataset. }
\end{table*}

%%%%%%%%%%%%%%%%%%%%%%%%%%%%%%%%%%%%%%%%%%%%%%%%%%%%%%%%%%%%%%%%%%%%%%%%%%%%%%%%%%%%%%%%%%%%%%%
%%%%% kitti model on apollo
%%%%%%%%%%%%%%%%%%%%%%%%%%%%%%%%%%%%%%%%%%%%%%%%%%%%%%%%%%%%%%%%%%%%%%%%%%%%%%%%%%%%%%%%%%%%%%%
\begin{table*}[h]
    \scriptsize
    \centering
    \begin{tabular}{llllllllllllllll}
        \toprule
        \multicolumn{2}{c}{\multirow{2}{*} {Apollo dataset}} & \multicolumn{7}{c}{Rotation (inlier ratio, error median)} & \multicolumn{7}{c}{Translation (inlier ratio, error median)} \\
        \cmidrule(r){3-9} \cmidrule(r){10-16} \\
        Catogories & KITTI Models & 0.01 & 0.02 & 0.05 & 0.1 & 0.5 & Mean & Med. & 0.1 & 0.2 & 0.5 & 1.0 & 2.0 & Mean & Med. \\
        \midrule

\textbf{Si-base} 
& Si-Ran & 0.058 & 0.227 & 0.662 & 0.922 & 0.997 & 0.157 & 0.037 & 0.065 & 0.214 & 0.623 & 0.890 & 0.979 & 0.788 & 0.388
\\ \midrule % \hline
\textbf{Sp-base} 
& Sp-Ran & 0.001 & 0.012 & 0.114 & 0.407 & 0.962 & 0.205 & 0.118 & 0.003 & 0.016 & 0.089 & 0.271 & 0.583 & 5.645 & 1.670
\\ \midrule % \hline
\textbf{Si-models} 
& Si-Df-f & 0.043 & 0.187 & 0.567 & 0.845 & 0.963 & 0.172 & 0.043 & 0.093 & 0.246 & 0.593 & 0.791 & 0.895 & 2.452 & 0.389
\\  % \hline
& Si-Df-p & 0.035 & 0.132 & 0.451 & 0.727 & 0.904 & 0.333 & 0.056 & 0.053 & 0.156 & 0.425 & 0.614 & 0.760 & 4.918 & 0.658
\\ % \hline
& Si-Df-fp & 0.040 & 0.169 & 0.561 & 0.840 & 0.971 & 0.148 & 0.044 & 0.098 & 0.271 & 0.608 & 0.807 & 0.911 & 2.103 & 0.369
\\ \midrule % \hline
\textbf{Sp-models} 
& Sp-Df-f & 0.005 & 0.041 & 0.315 & 0.725 & 0.989 & 0.126 & 0.068 & 0.007 & 0.032 & 0.155 & 0.425 & 0.754 & 2.074 & 1.155
\\ % \hline
& Sp-Df-p & 0.004 & 0.040 & 0.329 & 0.730 & 0.989 & 0.124 & 0.067 & 0.009 & 0.036 & 0.192 & 0.513 & 0.827 & 1.905 & 0.974
\\ \midrule % \hline
\texttt{DeepFEPE} 
& Sp-Df-f-end  & 0.012 & 0.088 & 0.487 & 0.841 & 0.992 & 0.100 & 0.051 & 0.025 & 0.092 & 0.416 & 0.750 & 0.910 & 1.122 & 0.589
\\ 
& Sp-Df-p-end & 0.007 & 0.040 & 0.305 & 0.686 & 0.963 & 0.152 & 0.071 & 0.007 & 0.028 & 0.187 & 0.472 & 0.747 & 2.652 & 1.068
\\ 
& Sp-Df-fp-end & 0.013 & 0.081 & 0.489 & 0.864 & 0.995 & 0.092 & 0.051 & 0.012 & 0.057 & 0.332 & 0.738 & 0.924 & 1.275 & 0.659
\\ \bottomrule % \hline

    \end{tabular}
\caption{\label{tab:exp_ablation_ref_table} \textbf{KITTI model on Apollo dataset. The full table for rotation and translation error.} The set of models are trained in solely in KITTI dataset or ApolloScape dataset. }
\end{table*}
