# Supplementary material for: Deep Keypoint-Based Camera Pose Estimation with Geometric Constraints
Source: arXiv:2007.15122 source file (2020-07-29)

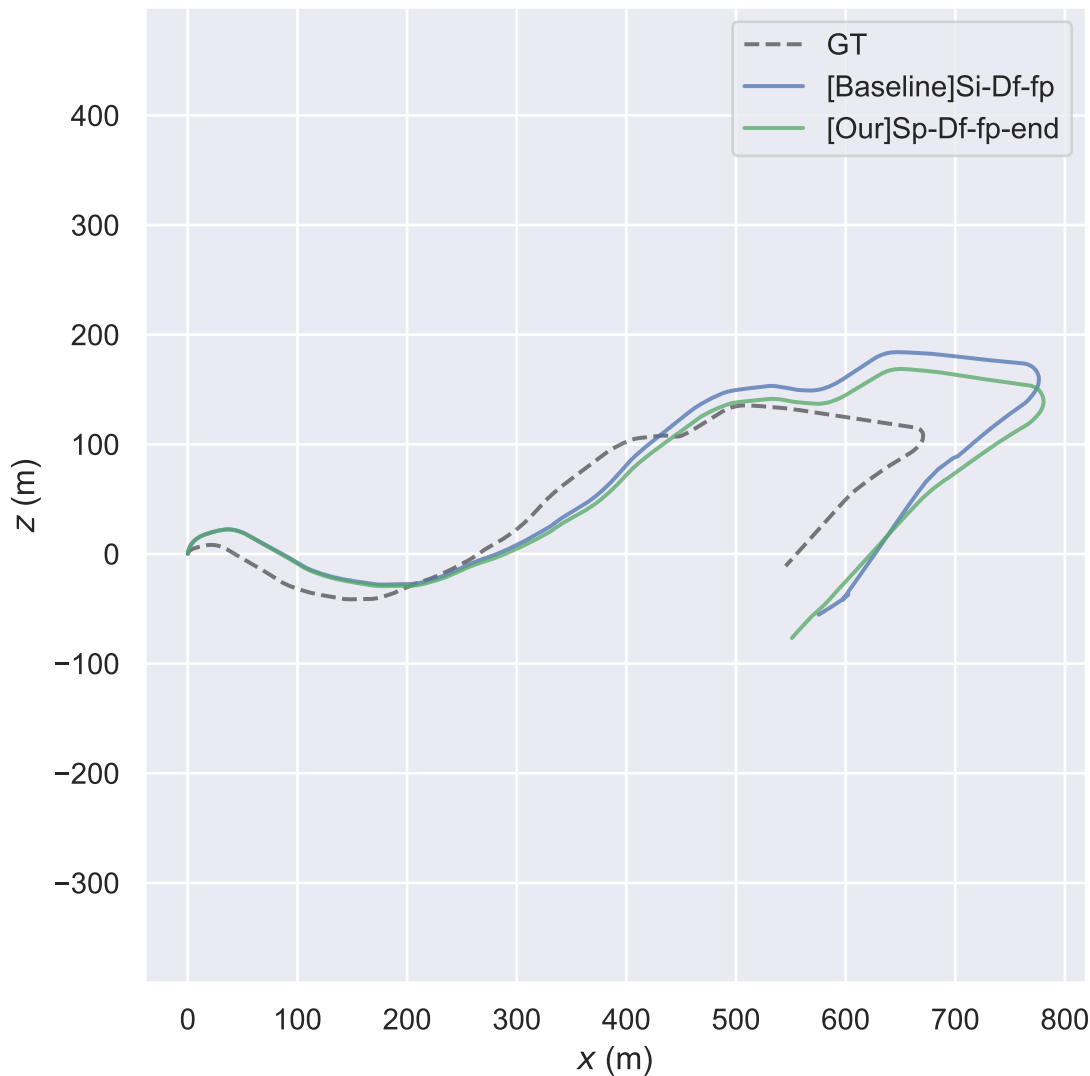

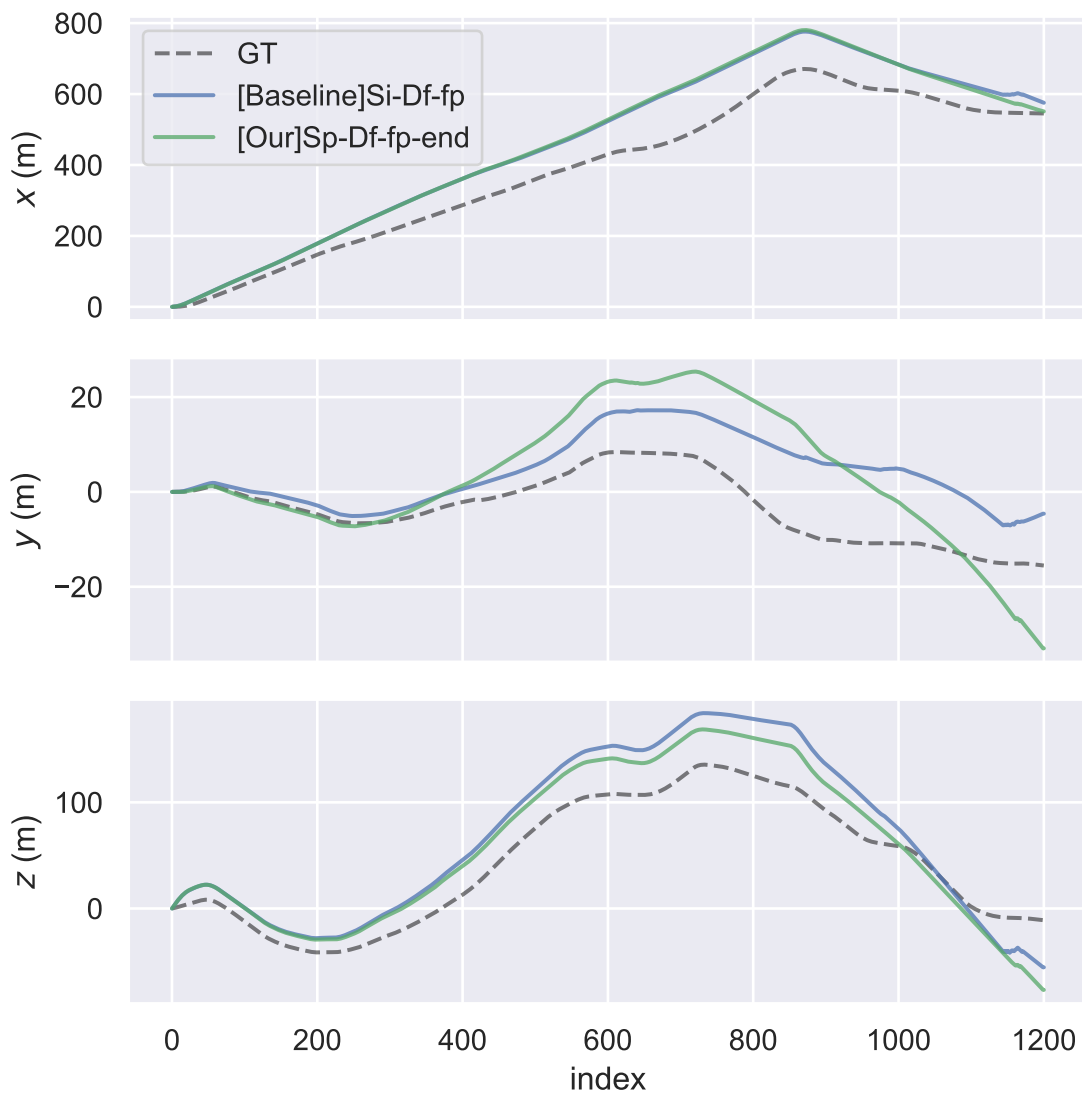

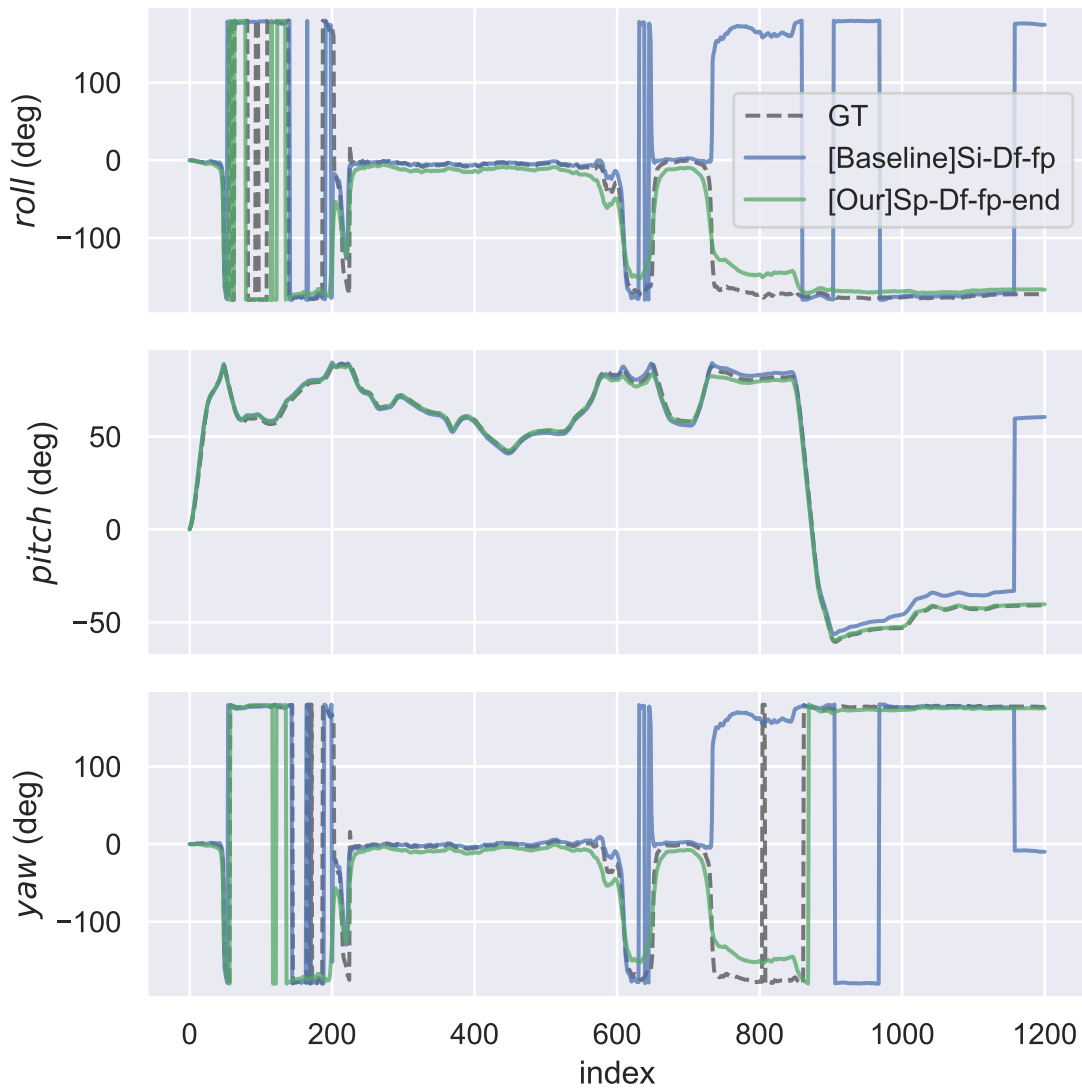

Supplement: Supplementary file 4 [file plot2curves_Si-D-k-f-p_k_1109_10_Sp-D-end-k-f-p_k_1109_10.pdf]
