# Supplementary material for: Deep Keypoint-Based Camera Pose Estimation with Geometric Constraints
Source: arXiv:2007.15122 source file (2020-07-29)
Supplement: Supplementary file 5 [file supp_ablation_apolloModels_smallTables.tex]

%%%% Apollo model (small tables) 

%%%% Apollo models - ours on apollo
% table: table_apolloModels_our_apo
\begin{table}[h]
    \scriptsize
    \centering
    \begin{tabular}{lllllll}
        \toprule
        \multirow{2}{*} {Apollo Models} & \multicolumn{6}{c}{Apollo dataset - error(deg.) inlier ratio$\uparrow$, mean$\downarrow$, median$\downarrow$}  \\
        \cmidrule(r){2-7}
        {}                               & \multicolumn{3}{c}{Rotation (deg.)} & \multicolumn{3}{c}{Translation (deg.)} \\
         {} & 0.1$\uparrow$  & Mean.$\downarrow$ & Med.$\downarrow$ & 2.0$\uparrow$ & Mean.$\downarrow$ & Med.$\downarrow$ \\
        \midrule

Base(Sp-Ran) & 0.320 & 0.271 & 0.138 & 0.489 & 5.887 & 2.044
\\ \hline
Sp-Df-f & 0.876 & 0.089 & 0.049 & 0.962 & 1.050 & 0.509
\\ \hline
Sp-Df-p & 0.865 & 0.091 & 0.050 & 0.964 & 1.052 & 0.497
\\ \hline
Ours(Sp-Df-f-end) & 0.914 & 0.084 & 0.044 & 0.976 & \textbf{0.774} & 0.443
\\ \hline
Ours(Sp-Df-p-end) & 0.900 & 0.086 & 0.046 & 0.977 & 0.805 & 0.421
\\ \hline
Ours(Sp-Df-fp-end) & \textbf{0.921} & \textbf{0.082} & \textbf{0.042} & \textbf{0.977} & 0.903 & \textbf{0.406}
\\ \hline

\bottomrule
    \end{tabular}
\caption{\label{tab:exp_ablation_apollo-apo-ours} \textbf{Comparison of pose estimation for our Apollo models on Apollo dataset.} 
The set of models are trained in Apollo dataset with learning-based feature extraction (FE). It shows improvement from RANSAC to DeepF pose estimation, and the benefits from separate models to end-to-end training. The end-to-end model shows the best mean and median errors.
}
% The table compares the learning based approaches in a cross dataset setting. The table shows that our end-to-end \texttt{DeepFEPE} performs the best.
\end{table}

%%%% Apollo models - baseline on apollo
% table: table_apolloModels_baselines_apo
\begin{table}[h]
    \scriptsize
    \centering
    \begin{tabular}{lllllll}
        \toprule
        \multirow{2}{*} {KITTI Models} & \multicolumn{6}{c}{Apollo dataset - error(deg.) inlier ratio$\uparrow$, mean$\downarrow$, median$\downarrow$}  \\
        \cmidrule(r){2-7}
        {}                               & \multicolumn{3}{c}{Rotation (deg.)} & \multicolumn{3}{c}{Translation (deg.)} \\
         {} & 0.1$\uparrow$  & Mean.$\downarrow$ & Med.$\downarrow$ & 2.0$\uparrow$ & Mean.$\downarrow$ & Med.$\downarrow$ \\
        \midrule

Base(Si-Ran) & 0.922 & 0.157 & 0.037 & 0.979 & 0.788 & 0.388
\\ \hline
Si-Df-f & 0.912 & \textbf{0.079} & 0.036 & 0.954 & 0.745 & 0.293
\\ \hline
Si-Df-p & \textbf{0.942} & 0.097 & \textbf{0.031} & \textbf{0.987} & \textbf{0.455} & \textbf{0.197}
\\ \hline
Ours(Sp-Df-fp-end) & 0.921 & 0.082 & 0.042 & 0.977 & 0.903 & 0.406
\\ \hline

\bottomrule
    \end{tabular}
\caption{\label{tab:exp_ablation_apollo-apo-base} \textbf{Comparison of pose estimation for Baseline Apollo models on Apollo dataset.} 
The table compares our best \texttt{DeepFEPE} model with SIFT based pose estimation. Our model performs on par with classic pipeline. The SIFT+DeepF pipeline is boosted with our geometry-based pose loss.
}
% The table compares our \texttt{DeepFEPE} with other baseline methods in a cross dataset setting. The results show that traditional method (SIFT + RANSAC) maintains the best overall results. Our model performs better than Si-models.
\end{table}

%%%% ours - kitti
% table: table_apolloModels_ours_kit
\begin{table}[h]
    \scriptsize
    \centering
    \begin{tabular}{lllllll}
        \toprule
        \multirow{2}{*} {Apollo Models} & \multicolumn{6}{c}{KITTI dataset - error(deg.) inlier ratio$\uparrow$, mean$\downarrow$, median$\downarrow$}  \\
        \cmidrule(r){2-7} 
        {}                               & \multicolumn{3}{c}{Rotation (deg.)} & \multicolumn{3}{c}{Translation (deg.)} \\
         {} & 0.1$\uparrow$  & Mean.$\downarrow$ & Med.$\downarrow$ & 2.0$\uparrow$ & Mean.$\downarrow$ & Med.$\downarrow$ \\
        \midrule
Base(Sp-Ran) & 0.190 & 0.820 & 0.224 & 0.472 & 7.142 & 2.162
\\ \hline
Sp-Df-f & 0.454 & 0.173 & 0.110 & 0.684 & 3.068 & 1.239
\\ \hline
Sp-Df-p & 0.424 & 0.170 & 0.118 & 0.699 & 2.442 & 1.190
\\ \hline
Ours(Sp-Df-f-end) & 0.529 & 0.135 & 0.094 & 0.767 & 2.454 & 1.032
\\ \hline
Ours(Sp-Df-p-end) & 0.467 & 0.159 & 0.106 & 0.750 & 2.466 & 1.112
\\ \hline
Ours(Sp-Df-fp-end) & \textbf{0.571} & \textbf{0.120} & \textbf{0.089} & \textbf{0.809} & \textbf{2.283} & \textbf{0.910}
\\ \hline

\bottomrule
    \end{tabular}
\caption{\label{tab:exp_ablation_apollo-kit-ours} \textbf{Comparison of pose estimation for learning-based Apollo models on KITTI dataset.} 
The table compares the learning-based models in a cross-dataset setting, which shows the clear gain from end-to-end training.
}
% The set of models are trained in KITTI with learning based feature extraction (FE). It shows significant improvement from RANSAC to DeepF pose estimation, and from separate models to end-to-end training.
\end{table}

%%%% baselines - kitti
% table: table_apolloModels_baselines_kit
\begin{table}[h]
    \scriptsize
    \centering
    \begin{tabular}{lllllll}
        \toprule
        \multirow{2}{*} {Apollo Models} & \multicolumn{6}{c}{KITTI dataset - error(deg.) inlier ratio$\uparrow$, mean$\downarrow$, median$\downarrow$}  \\
        \cmidrule(r){2-7} 
        {}                               & \multicolumn{3}{c}{Rotation (deg.)} & \multicolumn{3}{c}{Translation (deg.)} \\
         {} & 0.1$\uparrow$  & Mean.$\downarrow$ & Med.$\downarrow$ & 2.0$\uparrow$ & Mean.$\downarrow$ & Med.$\downarrow$ \\
        \midrule
Base(Si-Ran) & \textbf{0.818} & 0.391 & 0.056 & \textbf{0.899} & \textbf{1.895} & 0.639
\\ \hline
Si-Df-f & 0.706 & 0.130 & 0.066 & 0.824 & 3.133 & 0.686
\\ \hline
Si-Df-p & 0.786 & \textbf{0.096} & \textbf{0.054} & 0.860 & 1.932 & \textbf{0.606}
\\ \hline
Ours(Sp-Df-fp-end) & 0.571 & 0.120 & 0.089 & 0.809 & 2.283 & 0.910
\\ \hline

\bottomrule
    \end{tabular}
\caption{\label{tab:exp_ablation_apollo-kit-base} \textbf{Comparison of pose estimation for SIFT based Apollo models on KITTI dataset.} 
The table compares our best \texttt{DeepFEPE} model with SIFT based models.
}
% The table compare our best \texttt{DeepFEPE} model (End-to-end training with pose and F. loss) with SIFT based pose estimation. Our model works better than T-base, and comparable with state-of-the-art Si-models. 
\end{table}
